# Supplementary material for: Generative Adversarial Networks for Operational Scenario Planning of Renewable Energy Farms: A Study on Wind and Photovoltaic
Source: arXiv:1906.00662 source file (2019-06-03)
Supplement: Supplementary file 1 [file appendix.tex]

\begin{figure}[H]
\includegraphics[width=\linewidth]{figures/evaluation/dc_gan_48/pdfs_all.png}
\caption{Comparison of the estimated PDFs for the real and the generated samples over the whole training procress (generated using the DC-GAN).}
\end{figure}

\begin{figure}[H]
\includegraphics[width=\linewidth]{figures/evaluation/dc_wgan_48/pdfs_all.png}
\caption{Comparison of the estimated PDFs for the real and the generated samples over the whole training procress (generated using the DC-WGAN).}
\end{figure}
